# Supplementary material for: Solving reachability problems on data-aware workflows
Source: arXiv:1909.12738 source file (2020-09-03)
Supplement: Supplementary file 1 [file additional-backgrounds.tex]

\section{Preliminaries} \label{app:preliminaries}

\subsection{Workflow Nets}

\begin{definition}[Petri Net~\cite{de_leoni:2013}]
  A Petri Net is a triple $\tuple{P,T,F}$ where
  \begin{itemize}
    \item $P$ is a set of places;
    \item $T$ is a set of transitions;
    \item $F\subseteq (P \times T) \cup (T \times P)$ is the flow relation describing the ``arcs'' between places and transitions (and between transitions and places).
  \end{itemize}
  
  The \emph{preset} of a transition t is the set of its input places: $\pres{t} = \{p \in P \mid (p,t) \in F\}$. The \emph{postset} of $t$ is the set of its output places: $\posts{t} = \{p \in P \mid (t,p) \in F\}$. Definitions of pre- and postsets of places are analogous.
  
  The \emph{marking} of a Petri net is a total mapping $M : P\mapsto \mathbb{N}$.
\end{definition}

\begin{definition}[WF-net~\cite{sidorovastahletal:2011}]
A Petri net $\tuple{P,T,F}$ is a workflow net (WF-net) if it has a single source place start, a single sink place end, and every place and every transition is on a path from start to end; i.e.\ for all $n\in P\cup T$, $(start,n)\in F^*$ and $(n,end)\in F^*$, where $F^*$ is the reflexive transitive closure of $F$.
\end{definition}

The semantics of a PN is defined in terms of its markings and \emph{valid firing} of transitions which change the marking. A firing of a transition $t\in T$ from $M$ to $M'$ is valid -- denoted by $M \fire{t_0} M$ -- iff:
\begin{itemize}
  \item $t$ is enabled in $M$, i.e., $\{ p\in P\mid M(p)>0\}\supseteq \pres{t}$; and
  \item the marking $M'$ satisfies the property that for every $p\in P$:
  \begin{displaymath}
    M'(p) =
    \begin{cases}
      M(p)-1 & \text{if $p\in \pres{t}\setminus\posts{t}$}\\
      M(p)+1  & \text{if $p\in \posts{t}\setminus\pres{t}$}\\
      M(p) & \text{otherwise}
    \end{cases}
  \end{displaymath}
\end{itemize}
A \emph{case} of PN is a sequence of valid firings
$$M_0 \fire{t_1} M_1, M_1 \fire{t_2} M_2, \ldots, M_{k-1} \fire{t_k} M_k$$ where $M_0$ is the marking where there is a single token in the start place.

\begin{definition}[safeness]
 A marking of a Petri Net is $k$-safe if the number of tokens in all places is at most $k$. A Petri Net is $k$-safe if the initial marking is $k$-safe and the marking of all cases is $k$-safe. 
\end{definition}

In this document we focus on 1-safeness, which is equivalent to the original safeness property as defined in~\cite{vanderaalst:1998}.\footnote{In the following we will use safeness as a synonym of 1-safeness.} Note that for safe nets the range of markings is restricted to $\{0, 1\}$.

\subsection{Action Language \klng}

The formal definition of \klng can be found in Appendix A of~\cite{eiter_dlvk:2003}; here, as reference, we include the main concepts.

We assume disjoint sets of action, fluent and type names, i.e., predicate symbols of arity $\geq 0$, and disjoint sets of constant and variable symbols. Literals can be positive or negative atoms; denoted by $-$. Given a set of literals $L$, $L^+$ (respectively, $L^-$) is the set of positive (respectively, negative) literals in $L$. A set of literals is \emph{consistent} no atoms appear both positive and negated.

The set of all action (respectively, fluent, type) literals is denoted as $\L_{act}$ (respectively, $\L_{fl}$, $\L_{typ}$). 

Furthermore, $\L_{fl,typ} = \L_{fl} \cup \L_{typ}$, $\L_{dyn} = \L_{fl} \cup \L^+_{act}$, and $\L = \L_{fl,typ} \cup \L^+_{act}$.

\begin{definition}[Causation rule]
  A (causation) rule is an expression of the form
    \begin{lstlisting}
caused $f$ if $b_1,\ldots, b_k$, not $b_{k+1}$, $\ldots$, not $b_\ell$ 
         after $a_1,\ldots, a_m$, not $a_{m+1}$, $\ldots$, not $a_n$.
  \end{lstlisting}
were $f\in \L_{fl}\cup \{ false \}$, $b_i\in\L_{fl,typ}$, $a_i\in\L$, $\ell\geq k\geq 0$ and $n\geq m\geq 0$. 

If $n=0$ the rule is called \emph{static}.

We define $h(r) = f$, $pre^+(r) = \{a_1,\ldots, a_m\}$, $pre^-(r) = \{a_{m+1},\ldots, a_n\}$, $post^+(r) = \{b_1,\ldots, b_k\}$, $post^-(r) = \{b_{k+1},\ldots, b_\ell\}$
\end{definition}

\begin{definition}[Initial state constraints]
  An initial state constraint is a static rule preceded by the keyword \lstinline|initially|.
\end{definition}

\begin{definition}[Executability condition]
  An executability condition e is an expression of the form
    \begin{lstlisting}
executable $a$ if $b_1,\ldots, b_k$, not $b_{k+1}$, $\ldots$, not $b_\ell$.
  \end{lstlisting}
were $a\in \L_{act}^+$, $b_i\in\L_{fl,typ}$, and $\ell\geq k\geq 0$.

We define $h(e) = a$, $pre^+(e) = \{b_1,\ldots, b_k\}$, and $pre^-(e) = \{b_{k+1},\ldots, b_\ell\}$
\end{definition}

Since in this document we're dealing with ground plans, for the definition of \emph{typed instantiation} the reader is referred to the original paper.

\begin{definition}[Planning domain, \cite{eiter_dlvk:2003} Def.\ A.5]
An action description $\tuple{D,R}$ consists of a finite set $D$ of action and fluent declarations and a finite set $R$ of safe causation rules, safe initial state constraints, and safe executability conditions. A \klng planning domain is a pair $PD = \tuple{\Pi,AD}$, where $\Pi$ is a stratified Datalog program (the background knowledge) which is safe, and $AD$ is an action description. We call $PD$ positive, if no default negation occurs in AD.
\end{definition}

The set $lit(PD)$ contains all the literals appearing in PD.

\begin{definition}[State, State transition]
A state w.r.t.\ a planning domain PD is any consistent set $s\subseteq\L_{fl} \cap (lit(PD) \cup lit(PD)^-)$ of legal fluent instances and their negations. A state transition is any tuple $t = \tuple{s, A, s'}$ where $s, s'$ are states and $A \subseteq \L_{act} \cap lit(PD)$ is a set of legal action instances in PD.
\end{definition}

Semantics of plans including default negation is defined by means of a Gelfond–Lifschitz type reduction to a positive planning domain.
\begin{definition}
  Let PD be a ground and well-typed planning domain, and let $t = \tuple{s,A,s'}$ be a state transition. Then, the reduction $PD^t$ of PD by $t$ is the planning domain where the set of rules $R$ of PD is substituted by $R^t$ obtained by deleting
  \begin{enumerate}
    \item each $r\in R$,where either $post^-(r) \cap s'\neq\emptyset$ or $pre^-(r)\cap s\neq\emptyset$,and
    \item all default literals \lstinline|not $\ell$| ($\ell\in\L$) from the remaining $r\in R$.
  \end{enumerate}
\end{definition}

\begin{definition}[Legal initial state, executable action set, legal state transition]
For any planning domain $PD = \tuple{D,R}$
\begin{itemize}
  \item a state $s_0$ is a legal initial state, if $s_0$ is the least set s.t.\ for all static and initial rules $r$ $post(r)\subseteq s_0$ implies $h(r) \subseteq s_0$;
  \item a set $A\subseteq\L^+_{act}$ is an executable action set w.r.t.\ a state $s$, if for each $a\in A$ there is an executability condition $e\in R^{\tuple{s,A, \emptyset}}$ s.t.\ $h(e)=\{a\}$, $pre(e) \cap \L_{fl} \subseteq s$, and $pre(e) \cap \L^+_{act} \subseteq A$;
  \item a state transition $t = \tuple{s, A, s'}$ is legal if $A$ is an executable action set w.r.t.\ $s$, and $s'$ is the minimal consistent set that satisfies all causation rules in $R^{\tuple{s,A, s'}}$ w.r.t.\ $s \cup A$. A causation rule $r \in  R^{\tuple{s,A, s'}}$, is satisfied if the three conditions
      \begin{enumerate}
        \item $post(r) \subseteq s'$
        \item $pre(r) \cap \L_{fl} \subseteq s$
        \item $pre(r) \cap \L_{act} \subseteq A$
      \end{enumerate}
      all hold, then $h(r) \neq \{false\}$ and $h(r) \subseteq s'$.
\end{itemize}
\end{definition}

\begin{definition}[Trajectory]
A sequence of state transitions $$\tuple{s_0, A_1, s_1}, \tuple{s_1, A_2, s_2}, \ldots,\tuple{s_{n-1}, A_n, s_n}$$, $n \geq 0$, is a trajectory for PD, if $s_0$ is a legal initial state of PD and all $\tuple{s_{i-1}, A_i, s_i}$, $1\leq i\leq n$, are legal state transitions of PD.

If $n = 0$, then the trajectory is empty.
\end{definition}

\begin{definition}[Planning problem]
  A planning problem is a pair of planning domain PD and a ground goal $q$
    \begin{lstlisting}
$g_1,\ldots, g_m$, not $g_{m+1}$, $\ldots$, not $g_n$.
  \end{lstlisting}
where $g_i\in\L_{ft}$ and $n\geq m\geq 0$.

A state $s$ \emph{satisfies} the goal if $\{g_1,\ldots, g_m\}\subseteq s$ and $\{g_{m+1},\ldots, g_n\}\cap s = \emptyset$.
\end{definition}

\begin{definition}[Optimistic plan]
  A sequence of action sets $A_1,\ldots, A_k$ is an optimistic plan for a planning problem $\tuple{PD, q}$ if there is a trajectory $\tuple{s_0, A_1, s_1}, \ldots,\tuple{s_{k-1}, A_k, s_k}$ establishing the goal $q$, i.e.\ $s_k$ satisfies $q$.
\end{definition}

\begin{definition}[Secure plan]
  An optimistic plan $A_1,\ldots, A_n$ is secure if for every legal initial state $s_0$ and trajectory $\tuple{s_0, A_1, s_1}, \tuple{s_1, A_2, s_2}, \ldots,\tuple{s_{k-1}, A_k, s_k}$ $0\leq k\leq n$, it holds that
  \begin{enumerate}
    \item if $k=n$ then $s_k$ satisfies the goal;
    \item if $k<n$, then there is a legal transition $\tuple{s_k,A_{k+1},s_{k+1}}$.
  \end{enumerate}
\end{definition}

\nocite{vazquez:2014,eiter_dlvk:2003}

%%% Local Variables:
%%% mode: latex
%%% TeX-master: "DataWFNets-planning.tex"
%%% save-place: t
%%% End:
