# Supplementary material for: Solving reachability problems on data-aware workflows
Source: arXiv:1909.12738 source file (2020-09-03)
Supplement: Supplementary file 3 [file additional-framework.tex]

\section{Framework}

\subsection{Data Model}\label{sec:datamodel}

\begin{definition}[Data model]
A data model for is a couple $\D = (\V, \Delta, \domf, \ordf)$ where:
\begin{compactitem}
\item $\V$ is a possibly infinite set of variables;
\item $\Delta = \set{\Delta_1, \ldots, \Delta_n}$ is a set of domains (not necessarily disjoints);
\item $\domf: \V \rightarrow \Delta$ is a total and surjective function which associate to each variable $v$ its finite domain $\Delta_i$;
\item $\ordf$ is a partial function that, given a domain $\Delta_i$, if $\ordf(\Delta_i)$ is defined, then it returns a \emph{partial order} (reflexive, antisymmetric and transitive) $\leq_{\Delta_i} \subseteq \Delta_i \times \Delta_i$.
\end{compactitem}
\end{definition}

\begin{definition}[Assignment]
Let $\D = \tuple{\V, \Delta, \domf, \ordf}$ be a data model. An assignment for variables in $\V$ is a \emph{partial} function $\assign: \V \rightarrow \Delta_v$ such that for each $v \in \V$, if $\assign(v)$ is defined, then we have $\assign(v) \in \domf(v)$. We write $\Phi[\assign]$ for the formula $\Phi$ where each occurrence of a variable $v \in \img(\assign)$ is replaced by $\assign(v)$.
\end{definition}

\begin{definition}[Guard language, syntax]
Given a data model, the language $\guardlang$ of guards is the set of formulas $\Phi$ inductively defined according to the following grammar:
\[ \begin{array}{lcl}
\Phi & := & true \mid \deff(v) \mid t_1 = t_2 \mid t_1 \leq t_2 \mid \neg \Phi_1 \mid \Phi_1 \land \Phi_2
\end{array} \]
where $v \in \V$ and $t_1, t_2 \in \V \cup \bigcup_i \Delta_i$.
\end{definition}

\begin{definition}[Guard language, semantics]
Given a data model $\dmodel$, an assignment $\assign$ and a guard $\Phi \in \guardlang$ we say that $\dmodel, \assign$ satisfies $\Phi$, written $D, \assign \models \Phi$ inductively on the structure of $\Phi$ as follows:
\begin{itemize}
\item $\dmodel, \assign \models true$;
\item $\dmodel, \assign \models \deff(v)$ iff $v \in \img(\assign)$;
\item $\dmodel, \assign \models t_1 = t_2$ iff $t_1[\assign], t_2[\assign] \not \in \V$ and $t_1[\assign] \equiv t_2[\assign]$;
\item $\dmodel, \assign \models t_1 \leq t_2$ iff $t_1[\assign], t_2[\assign] \in \Delta_i$ for some $i$ and $\ordf(\Delta_i)$ is defined and $t_1[\assign] \leq_{\Delta_i} t_2[\assign]$;
\item $\dmodel, \assign \models \neg \Phi$ iff it is not the case that $\dmodel, \assign \models \Phi$;
\item $\dmodel, \assign \models \Phi_1 \land \Phi_2$ iff $\dmodel, \assign \models \Phi_1$ and $\dmodel, \assign \models \Phi_2$.
\end{itemize} 
\end{definition}

\subsection{Petri Nets with Data}\label{sec:our-net}

\begin{definition}[\ournet] 
  A Petri Net with data is a tuple $\tuple{\dmodel, \nmodel, \writef, \guardf}$ where:
\begin{itemize}
    \item $\nmodel=\tuple{P,T,F}$ is a Petri Net;
    \item $\dmodel=\tuple{\V, \Delta, \domf, \ordf}$ is a data model;
    \item $\writef: T \mapsto (\V' \mapsto 2^{\domf(\varset)})$, where $\varset'\subseteq\varset$ and $\writef(t)(v)\subseteq\domf(v)$ for each $v\in \varset'$, is a function that associate each transition to a (\emph{partial}) function mapping variables to a subset of their domain.
    \item $\guardf: T \mapsto \guardlang$ a function that associates a guard expression to each transition.
  \end{itemize}
\end{definition}

The definition of $\writef$ provides a fine grained description of the way that transitions modify the state of the \ournet, enabling the description of different cases:
\begin{itemize}
  \item $\emptyset\subset \writef(t)(v) \subseteq \domf(v)$: transition $t$ nondeterministically assigns a value from $\writef(t)(v)$ to $v$;\footnote{Allowing a subset of  $\domf(v)$ enables the specification of restrictions for specific tasks, e.g., while a task selects among \texttt{yes, no, maybe} another one can only choose between \texttt{yes} and \texttt{no}.}
  \item $\writef(t)(v) = \emptyset$: transition $t$ deletes the value of $v$ (undefined);
  \item $v \not\in dom(\writef(t))$: value of $v$ is not modified by transition $t$.
\end{itemize}

\begin{definition}
A state of a \ournet $\tuple{\dmodel, \nmodel, \writef, \guardf}$ is a pair $(\mrk,\assign)$ where $\mrk$ is a marking for $\tuple{P,T,F}$ and $\assign$ is an assignment. State transitions and firing are adapted to the additional information about data.
\end{definition}

\begin{definition}[Valid Firing]\label{def:dpn:firing}
  Given a \ournet $\tuple{\dmodel, \nmodel, \writef, \guardf}$, a firing of a transition $t\in T$ is valid firing in $(\mrk,\assign)$ resulting in a state $(\mrk',\assign')$ (written as $(\mrk,\assign)\fire{t}(\mrk',\assign')$) iff:
  \begin{itemize}
  \item $t$ is enabled in $\mrk$, i.e., $\{ p\in P\mid \mrk(p)>0\}\supseteq \pres{t}$; and
  \item $\dmodel, \assign \models \guardf(t)$;
  \item the marking $\mrk'$ satisfies the property that for every $p\in P$:
  \begin{displaymath}
    \mrk'(p) =
    \begin{cases}
      \mrk(p)-1 & \text{if $p\in \pres{t}\setminus\posts{t}$}\\
      \mrk (p)+1  & \text{if $p\in \posts{t}\setminus\pres{t}$}\\
      \mrk (p) & \text{otherwise}
    \end{cases}
  \end{displaymath}
  \item the assignment $\assign'$ satisfies the properties that its domain is $$dom(\assign') = dom(\assign)\cup\set{v\mid \writef(t)(v)\neq\emptyset}\setminus\set{v\mid \writef(t)(v)=\emptyset}$$ and for each $v\in dom(\assign')$:
  \begin{displaymath}
    \assign'(v) =
    \begin{cases}
      d \in \writef(t)(v) & \text{if $v\in dom(\writef(t))$}\\
      \assign(v)  & \text{otherwise.}
    \end{cases}
  \end{displaymath}
\end{itemize}
\end{definition}

Cases of \ournet are defined as those of WF-nets, with the only difference that in the initial state the assignment is empty.

%%% Local Variables:
%%% mode: latex
%%% TeX-master: "DataWFNets-planning.tex"
%%% save-place: t
%%% End:
